# Supplementary material for: Properties of the gradient squared of the discrete Gaussian free field
Source: arXiv:2207.09401 source file (2023-11-07)
Supplement: Supplementary file 2 [file appendix.tex]

\section{Appendix}

\textcolor{red}{Ignore for the moment}

\subsection{Computation of variance}

Let us start by evaluating at $x=y$. Expression \eqref{eq:green_double_diff} then becomes
\[
    \nabla_i^{(1)}\nabla_j^{(2)} G_0(x,x) = -\frac14 \left[a(e_i-e_j) - a(e_i) - a(e_j) + a(0)\right] \ ,
\]
where $0$ in the argument of the potential kernel represents the point $(0,0)$ in $\Z^2$.



Evaluating at $y=x$, and using the well-known values for the potential kernel (see \citet[Section 15]{spitzer}), we have
\[
    \nabla_i^{(1)}\nabla_j^{(2)} G_0(x,x) = 
    \begin{dcases}
    \hfil \frac12 \ &\text{if} \ i=j \ ,\\
    \frac12 - \frac1\pi \ &\text{if} \ i\neq j \ ,
    \end{dcases}
\]
for all $x\in\Z^2$. Using \eqref{eq:green_diff}, for all $x \in U$ we have
\[
    \lim_{\eps\to0} \nabla_i^{(1)}\nabla_j^{(2)} G_{U_\eps}\left(\floor{x/\eps},\floor{x/\eps}\right) = 
    \begin{dcases}
    \hfil \frac12 \ &\text{if} \ i=j \ ,\\
    \frac12 - \frac1\pi \ &\text{if} \ i\neq j \ .
    \end{dcases}
\]
Finally, \eqref{eq:limit_variance} reads
\begin{equation}\label{eq:conv_less_eps}
    \left[2\pi - 4 \left(1 - \frac1\pi\right)\right] \int_U f(x)^2 \, \d x = \left[2\pi - 4 \left(1 - \frac1\pi\right)\right] \norm{f}_{L^2} \ .
\end{equation}
